# Supplementary material for: Unsupervised Information Obfuscation for Split Inference of Neural Networks
Source: arXiv:2104.11413 source file (2021-06-23)
Supplement: Supplementary file 1 [file 6_Appendix.tex]

\appendix
\section{Appendix}

\begin{table}[ht]
\centering
\caption{\small Network Architecture. Each row shows a  split layer, e.g., at layer $1$, the raw data and, at layer $6$, the input to the last fully-connected layer is sent to the server.}\label{tab:architecture}
\resizebox{0.8\columnwidth}{!}{
\begin{tabular}{ccccc}
\textbf{Split Layer} &             &         &                   &                     \\ \hline
\textbf{1}     & CONV ($3,16$) & ReLU    & Max-Pooling ($2\times 2$) & Batch-Normalization \\ \hline
\textbf{2}     & CONV($3,32$)  & ReLU    & Max-Pooling ($2\times 2$) & Batch-Normalization \\ \hline
\textbf{3}     & CONV ($3,64$) & ReLU    & Max-Pooling ($2\times 2$) & Batch-Normalization \\ \hline
\textbf{4}     & FC(128)     & ReLU    & -                 & Batch-Normalization \\ \hline
\textbf{5}     & FC(64)      & ReLU    & -                 & Batch-Normalization \\ \hline
\textbf{6}     & FC(n\_classes)       & Softmax & -                 & -                  
\end{tabular}
}
\vspace{-0.25cm}
\end{table}

\begin{table}[ht]
\caption{\small Model accuracy for public and private attributes of different datasets.}\label{tab:baseline-accs} 
\centering
\resizebox{\columnwidth}{!}{
\begin{tabular}{c|c|c|c|cccccc}
\textbf{Dataset}               & MNIST  & UTKFace & FaceScrub & \multicolumn{6}{c}{CelebA}                                        \\ \hline
\textbf{number of classes}           & 10     & 2       & 2         & \multicolumn{6}{c}{2}                                             \\
\textbf{public attribute}      & digit  & gender  & gender    & \multicolumn{6}{c}{smiling}                                       \\
\textbf{public accuracy (\%)}  & 98.60  & 90.25   & 97.90     & \multicolumn{6}{c}{92.25}                                         \\ \hline
\textbf{number of classes}           & 100    & 5       & 530       & 2      & 2      & 2          & 2          & 2        & 2          \\
\textbf{private attribute}     & writer & race    & identity  & gender & makeup & cheekbones & mouth-open & lipstick & attractive \\
\textbf{private accuracy (\%)} & 26.93  & 79.18   & 65.52     & 97.53  & 90.00  & 86.29      & 92.94      & 93.40    & 80.46     
\end{tabular}
}
\vspace{-0.25cm}
\end{table}
