# Supplementary material for: Unsupervised Information Obfuscation for Split Inference of Neural Networks
Source: arXiv:2104.11413 source file (2021-06-23)
Supplement: Supplementary file 3 [file 7_Appendix_ICML_.tex]

\appendix

\section{Additional Experiments}
% \noindent{\bf Results for All Layers.} 
\textcolor{red}{Figure~\ref{fig:pub-priv-tradeoff} showed the effect of $m'$ on target and attack accuracy when splitting the network at the $FC1$ layer. Here we present in Figure~\ref{fig:all_layers} the effect of $m'$ for different split layers. As seen, the trend is similar in all split layers; that is, higher $m'$ results in higher target and attack accuracy.}

\begin{figure*}[h]
    \centering
    % \vspace{-0.1cm}
    \includegraphics[width=0.94\textwidth]{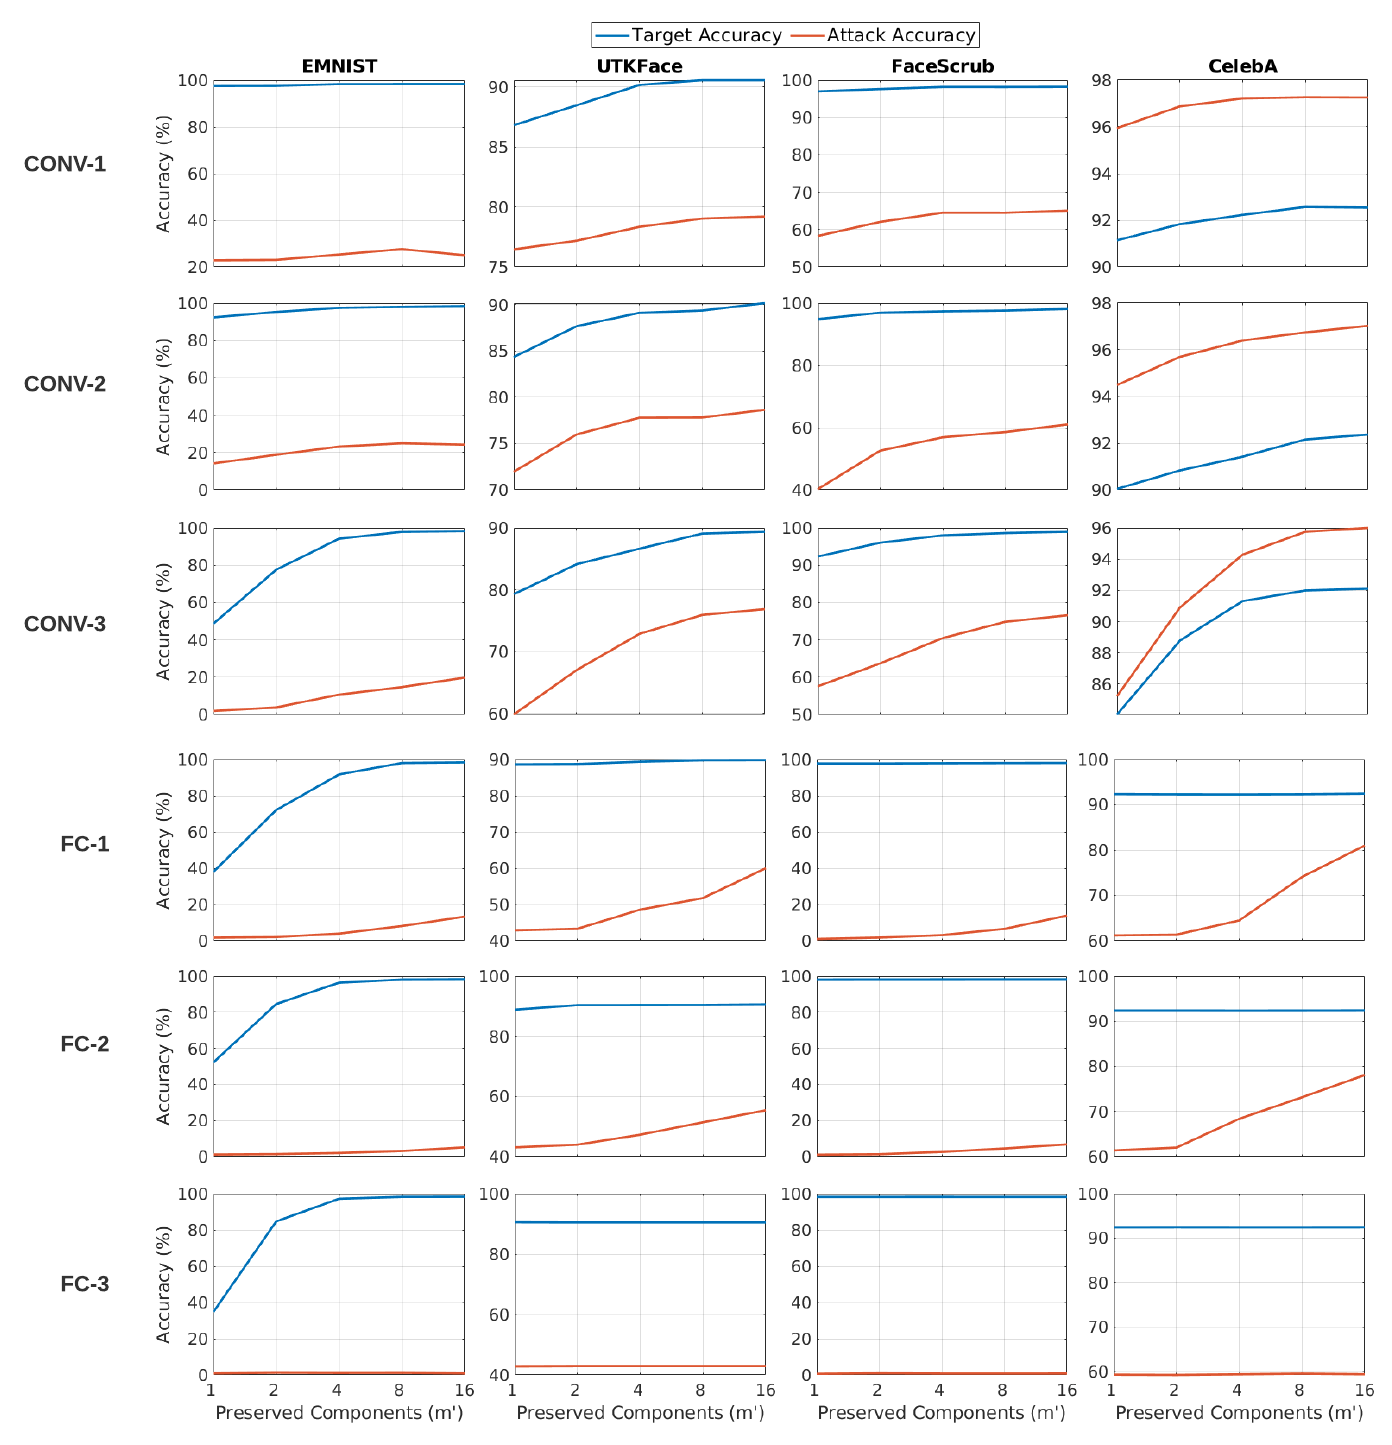}
    % \vspace{-0.5cm}
    \caption{\small Target and attack accuracy versus the number of preserved features, $m'$, for different split layers.}\label{fig:all_layers}
    % \vspace{-0.25cm}
\end{figure*}
